# Supplementary material for: Truthful Multi-Parameter Auctions with Online Supply: an Impossible Combination
Source: arXiv:1511.03699 source file (2017-07-14)
Supplement: Supplementary file 1 [file appendix.tex]

%appendix

\section{Missing Proofs}
\label{app:proofs}
